# Supplementary material for: Verifying Classification with Limited Disclosure
Source: arXiv:2502.16352 source file (2025-02-22)
Supplement: Supplementary file 1 [file apx_average_margin_genralized_skew_obtuse.tex]

\subsection{Possible New Lemma}

\begin{lemma}[New Robust Generalized Skew-Obtuse Family of Vectors]
\label{lemma:new_generalized-skew-obtuse_lemma}
    Let $V= \bar{v}_1,\bar{v}_2,\cdots, \bar{v}_k$ be a $k$ unit vectors in $\R^d$. Further, let  $W = w_1,w_2,\cdots, w_k$ be $k$ other unit vectors in $\R^d$. Suppose there exists $\alpha,\beta\in [0,1]$ and an error parameter $L$ such that the following holds:
    \begin{enumerate}
        \item for an $i$ chosen uniformly from $[k]$ we have $\E[\inner{\bar{v}_i}{w_i}] \geq \alpha$ and
        % \item for all $j\in [k]$ we have $\left|i\in[k]\colon  \inner{\bar{v}_i}{w_j} \leq -\beta\right|\geq k-1-L$. 
        \item there is a set $G$ of pairs $(i,j)$ with $i\neq j$ of size at least $k(k-1-L)$ such that the when picking $i,j$ uniformly from $G$ we have $\E[\inner{\bar{v}_i}{w_j}] \leq -\beta$
    \end{enumerate}
     Then, if $\alpha+2\beta>1$ we have $ k \leq \frac{(2+2L)(1+\beta)}{\alpha+2\beta-1}.$
     % Further if $\gamma=1/3$, there exists a skew-obtuse family of vectors with $k\geq \Omega(d)$ and if $\gamma<1/3$ then with $k\geq \exp{(\Omega_{1/3-\gamma}(d))}$.
\end{lemma}
